# Supplementary material for: MARVEL: Multidimensional Abstraction and Reasoning through Visual Evaluation and Learning
Source: arXiv:2404.13591 source file (2024-04-24)
Supplement: Supplementary file 1 [file error.tex]

\section{Example of Error Case}
\label{app: error}
